# Supplementary material for: Learning Dynamical Systems with Side Information
Source: arXiv:2008.10135 source file (2022-01-17)
Supplement: Supplementary file 1 [file appendix.tex]

\appendix

\section{Proof of \crec{prop:equivalence-metric-vf}}
For the proof, we need the following lemma first.

\begin{lemma}[Gronwall]
  Let $I = [a, b]$ denote a non-empty interval on the real line. Let
  $\alpha$, $\beta,$ and $u$ be continuous, real-valued functions
  defined on $I$ and satisfying
  \[u(t) \le \alpha(t) + \int_a^t \beta(s) u(s) \; {\rm d}s \quad
    \forall t \in I.\] If $\alpha$ is nondecreasing and $\beta$ is
  nonnegative, then
  \[u(t) \le \alpha(t) \exp\left(\int_a^t \beta(s) \; {\rm d}s\right)
    \quad t \in I.\]
\end{lemma}
\begin{proof}
  Consider two trajectories $\ix$ and $\iy$ both starting from
  $\ix_0 \in \Omega$ and following $f$ and $g$ respectively. Since
  $\ltwonorm{\dot \ix(0, \ix_0) - \dot \iy(0, \ix_0)} =
  \ltwonorm{f(\ix_0) - g(\ix_0)}$, the metric
  $\metricdyn{\cdot}{\Omega}{T}$ is bounded below by
  $\metricsup{\cdot}{\Omega}$.

  Let us now prove that 
  For the first part of the proof, we will bound $\|y(t) - x(t)\|$. By definition of $y$ and $x$, for every $t \in [0, T]$ we have that
  \begin{align*}
    x(t) - y(t) &= \int_0^t  f(x(s)) - g(y(s)) {\rm d}s
                  \\&= \int_0^t  f(x(s)) - g(x(s))\; {\rm d}s +  \int_0^t g(x(s)) - g(y(s)) \; {\rm d}s.
  \end{align*}

  Using the triangular inequality
  \begin{align}\label{eq:tirang_ineq}
    \|y(t) - x(t)\| & \le  \int_0^t  \|f(x(s)) - g(x(s))\|\; {\rm d}s +  \int_0^t \|g(x(s)) - g(y(s))\| \; {\rm d}s.
  \end{align}
  Since $f$ leaves $\Omega$ invariant, we know that for all $s \in [0, t]$, $x(s) \in \Omega$ and therefore $\|f(x(s)) - g(x(s))\| \le \metricsup{f-g}{\Omega}$. Furthermore, because the function $g$ is $L\text{-Lipchiz}$, $\|g(x(s)) - g(y(s))\| \; {\rm d}s \le L \|x(s) - y(s)\|$. From \eqref{eq:tirang_ineq} we conclude therefore that
  \begin{align*}
    \|y(t) - x(t)\| & \le  t \metricsup{f-g}{\Omega} + L \int_0^t  \|x(s) - y(s)\| \; {\rm d}s,
  \end{align*}
  and by Gronwall's lemma, 
  \[\|y(t) - x(t)\| \le  t \exp(Lt) \metricsup{f-g}{\Omega}\; \forall t \in [0, T].\]

  For the second part of the proof, we will bound $\|\frac{\partial}{\partial t}y(t) - \frac{\partial}{\partial t}x(t)\| = \|f(x(s)) - g(y(s))\|$.  note that since $f$ and $g$ leave $\Omega$ invariant, we know that for all $s \in [0, t]$, $x(s), y(s) \in \Omega$. By triangular inequality again, we know that $\|f(x(s)) - g(y(s))\| \le \|f(x(s)) - g(x(s))\| + \|g(x(s)) - g(y(s))\|$. Using the fact that $g$ is  $L\text{-Lipchiz}$ on $\Omega$,  $\|g(x(s)) - g(y(s))\| \le L\|y(t) - x(t)\|$. Therefore
  $\|f(x(s)) - g(y(s))\| \le \metricsup{f-g}{\Omega} + L\|y(t) - x(t)\|$.

  Putting the first and second part of the proof together, we have
  \[\|y(t) - x(t)\|  \le  T \exp(LT) \metricsup{f-g}{\Omega}\]
  and
  \begin{align*}
    \|\frac{\partial}{\partial t}y(t) - \frac{\partial}{\partial t}x(t)\|  & \le  \metricsup{f-g}{\Omega} + L\|y(t) - x(t)\|
    \\&\le \metricsup{f-g}{\Omega} + Lt \exp(Lt) \metricsup{f-g}{\Omega}.\\
  \end{align*}
  Therefore
  \[\metricdyn{f-g}{\Omega}{T} \le C(\Omega, T, L) \metricsup{f-g}{\Omega}\]
  with $C(\Omega, T, L) = \max\{T \exp(LT), 1+LT \exp(LT)\}$.
\end{proof}

Let $V$ be a  semialgebraic defined by $m$ polynomial inequalities $g_1(\x) \ge 0, \ldots, g_m(\x) \ge 0$. We consider the following regularity condition that should hold for any $\x \in V$,
\begin{align}
  &\inf_{\x, g_i(\x) = 0} \|\nabla g_i(\x)\| > 0 \quad i=1,\ldots,m\label{eq:grad_non_zero}\\
  &g_i(\x) = 0 \text{ and } |g_j(\x)| \le \eta  \implies  \langle \nabla g_i(\x), \nabla g_j(\x)\rangle \ge 0 \quad \forall \x \in V, \forall i, j =1,\ldots,m\label{eq:positive_cor_grad},
\end{align}
where $\eta$ is a positive constant independent of $\x$.

The next theorem states that under this regularity condition, any continuous vector field $f$ that leaves a semialgebraic set $V$ invariant can be approximated uniformly by polynomial vector field that leaves the set $V$ invariant as well.

\begin{theorem}
  Let $\Omega \subseteq \R^N$ be a compact subset of $\R^n$m and let $V \in \Omega$ be semialgebraic set satisfying the regularity conditions in \eqref{eq:grad_non_zero} and \eqref{eq:positive_cor_grad}. Consider a continuous vector field $f:\Omega\rightarrow \R^n$ that leaves the set $V$ invariant, i.e. $\forall \x \in V, g_i(\x) = 0 \implies \langle f(\x), \nabla g_i(\x) \ge 0$.

  For any $\varepsilon > 0$, there exists a polynomial $p \in \R[\x]$ such that for all $\x \in \Omega$:
  \[\ltwonorm{p(x) - f(x)} \le \varepsilon  \quad \text{ and } \quad \x \in V, \; g_i(\x) = 0 \implies \langle p(\x), \nabla g_i(\x) \ge 0 \text{for } i = 1,\ldots,m\].
\end{theorem}

\begin{proof}
  For the proof, we are going to use the following notation: 
  \[\lambda_i(\x) \coloneqq \exp(- \gamma g_j(\x)) \text{ for some $\gamma$ that we are going to fix later,}\]
  \[m_\nabla \coloneqq \min_i \min_{\x in V, g_i(\x) = 0} \|\nabla g_i(\x)\|,\]
  \[M_\nabla \coloneqq \max_{\x \in \Omega}\sum_{i=1}^m \|\lambda_i(\x)\nabla g_i(\x)\|.\]

  For $\alpha > 0$, let $\tilde f(\x) = f(\x) + \alpha \sum_{i=1}^m \lambda_i(\x) \nabla g_i(\x)$. This vector field $\tilde f$ is close to $f$, i.e.
  \[\|\tilde f(\x) - f(\x)\| \le \alpha M_\nabla.\]
  Let us now prove that for some choice of $\gamma$, $\tilde f$  leaves $V$ strictly invariant. For that, fix $x \in \Omega$ such that $g_i(\x) = 0$. We partition the set of indices $\{1, \ldots, n\}$ into three subsets
  $\{i\}$, $I^{[0, \eta]} = \{ j \ne i \; | ; |g_j(\x)| \le \eta \}$ and $I^{(\eta, \infty)} = \{ j \ne i \; | ; |g_j(\x)| > \eta\}$, so that we have
\[\begin{array}{ll}
    \lambda_i(\x) = 1\\
    \langle \nabla g_i(\x), \nabla g_j(\x) \rangle \ge 0 & \text{ for } j \in I^{[0, \eta]} \quad \text{by \eqref{eq:positive_cor_grad}}\\
    \lambda_j(\x) \le e^{-\gamma \eta} & \text{o.w.} \\
  \end{array}\]
  This implies the following inequalities
  \begin{align*}
    \langle \tilde f(\x), \nabla g_i(\x) \rangle
    &= \underbrace{\langle f(\x), \nabla g_i(\x) \rangle}_{ \ge 0} + \alpha \left(\|\nabla g_i(\x)\|^2 + \sum_{j \in I^{[0, \eta]}}\lambda_j(\x) \underbrace{\langle \nabla g_j(\x), \nabla g_i(\x) \rangle}_{\ge 0} + \sum_{j \in I^{(\eta, \infty)}}\underbrace{\lambda_j(\x)}_{\le e^{-\gamma \eta}} \langle \nabla g_j(\x), \nabla g_i(\x) \rangle\right)
    \\&\ge \alpha \left(\|\nabla g_i(\x)\|^2 - e^{-\gamma \eta}  \sum_{i=1}^m |\langle \nabla g_j(\x), \nabla g_i(\x) \rangle|\right)
    \\&\ge \alpha \left(m_\nabla - e^{-\gamma \eta}  \sum_{i=1}^m |\langle \nabla g_j(\x), \nabla g_i(\x) \rangle|\right)
  \end{align*}
  We can thus conclude that for  $\gamma$ large enough such that $e^{-\gamma \eta}  \max_{\x \in V} \sum_{i=1}^m |\langle \nabla g_j(\x), \nabla g_i(\x) \rangle| \le m_{\nabla}/2$, the quantity $\langle \tilde f(\x), \nabla g_i(\x) \rangle$ is at least $\alpha m_\nabla/2$.

In the rest of the proof, we will approximate $\tilde f$ by a polynomial $p$ and show that this polynomial also leaves the set $V$ invariant. Indeed, for any $\beta > 0$, using Weirstrass theorem, we can find a polynomial $p$ that satifies $\|\tilde f(\x) - p(\x)\| \le \beta$ for all $\x \in \Omega$. It follows that
  \[\|f(\x) - p(\x)\| \le \|f(\x) - \tilde f(\x)\| + \beta\]
  and
  \[\langle p(\x), \nabla g_i(\x) \ge \langle \tilde f (\x), \nabla g_i(\x)\rangle - \beta \|\nabla g_i(\x)\|.\]
  If we take \[\alpha = \varepsilon \min\{ \frac1{M_\nabla}, m_\nabla\} \text{ and } \beta = \frac{\varepsilon}{2 m_{\nabla}},\]
  then
  \[\|p(\x) - f(\x)\| \le 2\varepsilon \text{ and } g_i(\x) = 0 \implies \langle p(\x), \nabla g_i(\x) \ge \frac\varepsilon2.\]
  Which concludes the proof.
\end{proof}

%%% Local Variables:
%%% mode: latex
%%% TeX-engine: luatex
%%% TeX-command-extra-options: "-shell-escape"
%%% TeX-master: "Learning_with_side_information_v1"
%%% End:
